# Supplementary material for: Surprisingly-early bias in forecasts for unscheduled events
Source: arXiv:2512.07575 source file (2025-12-08)
Supplement: Supplementary file 1 [file Optimal_Calibration_1_1_Supplement_arXiV.pdf]

# Supplemental Materials

## Replicability

The full code for the simulation study is available at:

`https://github.com/PfadQualle/surprisingly_early_bias_replication`

The code should run in one minute or less on a standard modern personal computer. We remark that we simulate the data independently for the samples. As mentioned in the main text, we collect ten samples of the data in time at $t = \{0.1T, 0.2T, ..., 0.9T, T\}$. That is, the dataset is not one coherent history, but rather presents the outcomes of 10 independent simulations, each run to different points in time. This is not a problem for our analysis, but it means that the outcome of one event can change multiple times in the data.

No data for the analysis involving Metaculus data from section 3 is provided, as this data is owned by Metaculus, who generously made it available for the present analysis. The code, albeit useless without the data, is available upon reasonable request.

## Details related to the Metaculus dataset

Since the distinction in time-varying and time-fixed events is new, and not made in the Metaculus data, we classified all binary events by hand using the "resolution criteria" provided by the question authors. This led to an unambiguous classification in most cases. We applied the label "NA" to ambiguous resolution criteria. We exclude—from the Metaculus dataset—bias-inducing events where the early outcome could only be 'no' or 0. These introduce a surprisingly-early bias that is in the "opposite" direction. In order to make sure that the selection bias is going in one direction only, as in the simulation study from section 2, we simply excluded these events. There are only five such events in the dataset. Otherwise, we used all binary questions from the inception of the platform in 2015 until our data cutoff in August 2024. We reduce our analysis to binary forecasts (Metaculus also features density forecasts) in order to stay in line with the setup of section 2.

## Estimating the surprisingly-early bias in real world data

In the section 'Real-world forecasting data' the main text presents that "the observed frequency of events is on average 1.47 percentage points higher in the full dataset that is fraught with selection bias" and that "this is significantly different from zero ($p < 0.01$)". We explain this estimate here in more detail.

We kindly received the predictions data from Metaculus. Given that this data is not publicly available, this part of the article in not replicable and we provide no code.

We estimate the calibration of Metaculus forecasters by binning the reported predictions $q$ at the 0.01-level, i.e. $\{0.01, 0.02, ..., 0.99\}$. Then we observe the fraction of events for which the outcome was $X_i = 1$ or 'Yes' (relative to the total number of events), conditional on the respective prediction-levels. This gives us the frequency of events $\mu$ (vertical axis in Figure 3). We do this for two datasets of forecasts (including and excluding bias-inducing events), which yields us the two sets of calibration points featured in Figure 3. We indicate points from the dataset excluding/including bias-inducing events as $bias \in \{0; 1\}$ respectively. We fit a linear regression through each of the two sets of points. Specifically, we apply a weighted least squares model, where the weights correspond to the number of predictions in each bin. The regression model is shown in equation 1. We use standard standard errors.

$$\mu = \beta_0 + \beta_1\, q + \beta_2\, bias + \epsilon \qquad \mathbb{E}[\varepsilon_i \mid q,\ bias] = 0 \tag{1}$$

Thus, geometrically speaking, the dummy variable *bias* refers to the average change in frequency between the two fitted lines, or "how much parallel shift between the two calibration lines is". Table 1 reports results. We find that the fraction of outcomes verified to be $X_i = 1$ is 1.47% higher on average (across bins) in the biased dataset.

Table 1: Regression Estimates

| | **Estimate** | **std. error** | **t-value** |
|---|---|---|---|
| $\beta_0$ (Intercept) | -0.0123* | 0.0053 | -2.32 |
| $\beta_1$ ($q$) | 0.8791*** | 0.009 | 98.214 |
| $\beta_2$ ($bias$) | 0.0147** | 0.0056 | 2.614 |

Notes: * $p \leq 0.05$; ** $p < 0.01$; *** $p < 0.001$.
This table reports the coefficient estimates from applying a weighted least squares model to the calibration data from Metaculus. The hypothesis test for all coefficients is against 0.
